# Supplementary material for: Proactive DP: A Multple Target Optimization Framework for DP-SGD
Source: arXiv:2102.09030 source file (2024-06-04)
Supplement: Supplementary file 1 [file 07_Appendix.tex]

\section{Appendix K-Max Federated Learning}

We propose new algorithm which combines the global model by averaging k-model with highest accuracy (Experiments for k-max federated learning ($Figure$ 5) is shown from ($Figure$ 7 to $Figure$ 11). Specifically:

\begin{enumerate}[topsep=0pt,itemsep=-1ex,partopsep=1ex,parsep=1ex]
    \item A subset of clients is selected.
    
    \item Each client in the subset downloads \textbf{the current global model}.
    
    \item Each client in the subset computes \textbf{an updated model and a test accuracy} based on their local data.
    
    \item \textbf{The updated models and test accuracy} are sent from the selected clients to the sever.
    
    \item The server calculate \textbf{the average test accuracy, select a subset of model} (have their own accuracy larger than average accuracy) and average these models to construct an improved global model.
\end{enumerate}

\begin{table}[t]
\caption{Federated Learning Parameters}
\label{sample-table}
\vskip 0.15in
\begin{center}
\begin{small}
\begin{sc}
\begin{tabular}{lcccr}
\toprule
Parameter & Value & Notes \\ [0.5ex]
\midrule
Started learning rate & 0.01 &    \\ % inserting body of the table
Data Set & MNIST-Fashion & MNIST is too easy.   \\
Batch size & [32, 64] &                         \\
Number of epoch & [10, 20] &                    \\
Interval Step & 100 &                           \\
Number of workers & 24 &                        \\
Chosen K-Max Model & 7 &                        \\
Decaying step size & 100 &                      \\
Average running times & 8 &                     \\
\bottomrule
\end{tabular}
\end{sc}
\end{small}
\end{center}
\vskip -0.1in
\end{table}

\begin{figure}[!tbp]
  \centering
  \begin{minipage}[b]{0.45\textwidth}
    \includegraphics[width=\textwidth]{Figures/K-max_Average_Federate_Learning10.png}
    \caption{Test Accuracy, running time = 10}
    \label{fig:comfd1}
  \end{minipage}
  \hfill
  \begin{minipage}[b]{0.45\textwidth}
    \includegraphics[width=\textwidth]{Figures/K-max_Average_Federate_Learning20.png}
    \caption{Test Accuracy, running time = 20}
    \label{fig:comfd2}
  \end{minipage}
\end{figure}

% \begin{figure}
% \includegraphics[width=10cm, keepaspectratio]{Figures/K-max_Average_Federate_Learning10.png}
% \caption{Test Accuracy, running time = 10}
% \label{fig:comfd1}
% \end{figure}

% \begin{figure}
% \includegraphics[width=10cm, keepaspectratio]{Figures/K-max_Average_Federate_Learning20.png}
% \caption{Test Accuracy, running time = 20}
% \label{fig:comfd2}
% \end{figure}

\begin{figure}[!tbp]
  \centering
  \begin{minipage}[b]{0.55\textwidth}
    \includegraphics[width=\textwidth]{Figures/K-max_Average_Federate_Learning30.png}
    \caption{Test Accuracy, running time = 30}
    \label{fig:comfd3}
  \end{minipage}
  \hfill
  \begin{minipage}[b]{0.55\textwidth}
    \includegraphics[width=\textwidth]{Figures/K-max_Average_Federate_Learning50.png}
    \caption{Test Accuracy, running time = 50}
    \label{fig:comfd4}
  \end{minipage}
  \begin{minipage}[b]{0.55\textwidth}
    \includegraphics[width=\textwidth]{Figures/K-max_Average_Federate_Learning100.png}
    \caption{Test Accuracy, running time = 100}
    \label{fig:comfd5}
  \end{minipage}
\end{figure}
