# Supplementary material for: Proactive DP: A Multple Target Optimization Framework for DP-SGD
Source: arXiv:2102.09030 source file (2024-06-04)
Supplement: Supplementary file 3 [file appendix_C.tex]

\section{Differential Privacy Calculator}
\label{sec:dp_calculator}

\subsection{DP Calculator}
For each dataset, in order to achieving both accuracy and privacy, we need to find a set of parameters which provides at least 1.1 times the minimal accuracy and $(\epsilon,\delta)$ differential privacy. Therefore, we introduce DP-calculator which generates possible hyper-parameter settings based on \textbf{Theorem 6} and store them in tables. After that, we can perform queries on those tables to get a suitable hyper-parameter settings.

The goal of this calculator is finding the smallest accumulative noise $(\sigma \sqrt{T})$ and an increasing sample size sequence $s_i = q(i+m)^p$ given the following values: $p$, dataset size $N_c$, number of iterations $K$, privacy budget $(\epsilon,\delta)$, Gaussian noise ($\sigma$) and $\gamma$.

The DP calculator generates all possible valid sets of parameters and stores them in tables and then choose the best setting which has the smallest accumulative noise and privacy budget. In the tables generation process, there are four main steps described in the Figure \ref{fig:table_transformation}: 
     \begin{figure}[H]
        \centering
        \includegraphics[scale=0.15]{Figures/table_transformation_new.png}
        \caption{Table generation process example: Consider a dataset which has 60000 examples and we need 60000 iterations to train the model. Assuming with $\sigma \leq 20$ we can achieve the target accuracy, now we need to find the smallest privacy budgets $(\epsilon,\delta)$ which guarantees differential privacy.}
        \label{fig:table_transformation}
    \end{figure}

\begin{enumerate}
    \item \textbf{Generate Original Table}: First, we calculate the range of q based on theorem 6's case 1 ($K \leq min(K^-,K^*)$) and case 2 ($K^+ \leq K \leq K^*)$ for each setting ($p,N_c,K,\epsilon,\delta,\sigma,\gamma$) and construct the original table.

\begin{algorithm}
\caption{Constructing Original Table}
\label{alg:ConstructingOriginalTable}
\begin{algorithmic}[1]
    \Procedure{$construct\_ original\_table$}{$p,N_c,K,\epsilon,\delta,\sigma,\gamma$}
    \State {\bf Input:} \\
    \quad \textbullet \quad $p \in [0,1]$, Dataset Size ($N_c$), Number of iterations (K), \\ 
    \quad \textbullet \quad Privacy budget ($\epsilon,\delta$) \\
    \quad \textbullet \quad Gaussian Noise ($\sigma$),Gamma Value($\gamma$)
    \State {\bf Initialize:} 
    % \State $q\_interval_1 = (0,0]$
    % \State $q\_interval_2 = [\infty,0]$
    \State $q\_interval_1 = \oslash$
    \State $q\_interval_2 = \oslash$
    \For{$r_0 \in [0,\frac{1}{e}]$}
        
        \State $uq = \left[\frac{(r_0/\sigma)^\frac{1+p}{p}\cdot (1+\gamma)^{1+p} \cdot N_c}{(p+1) \cdot K}\right]^{p}$ 
        \Comment{$q \leq uq \iff K\leq K^*$}
        \State $r = calculate\_r(r_0,\sigma)$ 
        \If{$\sigma \geq \sqrt{\frac{2ln(1/\delta)}{\epsilon}} \cdot \frac{(1+\gamma)^{2+3p}}{\sqrt{1-r_0/\sigma}}$}
            \State $uq_1 = \left[\frac{B(r,p,r_0,\sigma) \cdot \epsilon^{(1+p)/(1+2*p)} \cdot N_c}{K}\right]^{1+2p}$ 
            \Comment{$q \leq uq_1 \iff K\leq K^-$}
            % \State $q\_interval_1= (0,max(min(uq,uq1),q\_interval_1[1])]$
            \State $q\_interval_1= q\_interval_1 \cup (0,min(uq,uq1)] $
        \EndIf
        \If{$r \geq \frac{\sqrt{\frac{2}{(1+\gamma)^{3+4p}} + 1}-1}{2} \cdot \frac{(3p+1}{(p+1)(2p+1)} \cdot \frac{(1-\alpha)^2}{(1+\gamma)^{2p}}$}
            \State $lq_2 = \left[\frac{A(r,p,r_0,\sigma) \cdot \epsilon^{(1+p)/(1+2*p)} \cdot N_c}{K}\right]^{1+2p}$ 
            \Comment{$q \geq lq_2 \iff K\geq K^+$}
            \State $C =\frac{2}{\sigma(1-\alpha)^{3/2}} \cdot \sqrt{r\frac{(p+1)(2p+1)}{3p+1}} \cdot \sqrt{\frac{2\ln{1/\delta}}{\epsilon}} \cdot (1 + \gamma)^{2(1+2p)}$ 
        
            \State $uq_2 = \left[\frac{A(r,p,r_0,\sigma)\cdot \epsilon^{(1+p)/(1+2p)} \cdot N_c}{K \cdot C^{(2+2p)/(1+2p)}}\right]^{1+2p}$
            % \Comment{Equation (18) inequality}
            \If{$lq2 <= uq$} \Comment{Case 2 exists}
                \State $q\_interval_2 = q\_interval_2 \cup [lq2,min(uq,uq2)]$
            \EndIf
        \EndIf
    \EndFor
    \State \Return $[[p,N_c,K],[\epsilon,\delta],[\sigma,\gamma],[q\_interval_1,q\_interval_2]]$
    \EndProcedure
\end{algorithmic}
\end{algorithm}
    \item \textbf{Compute $q_{max}$}: Next, we choose the maximum value of q in the computed intervals because the larger q is, the smaller T becomes:
    \begin{algorithm}[H]
        \caption{Compute $q_{max}$}
        \label{alg:ComputeQMax}
        \begin{algorithmic}[1]
            \Procedure{$compute\_q\_max$}{$p,N_c,K,\epsilon,\delta,\sigma,\gamma,[q\_interval_1,q\_interval_2]$}
            \State {\bf Input:} \\
            \quad \textbullet \quad $p \in [0,1]$, Dataset Size ($N_c$), Number of iterations (K)\\
            \quad \textbullet \quad Privacy budget ($\epsilon,\delta$) \\
            \quad \textbullet \quad Gaussian Noise ($\sigma$),Gamma Value($\gamma$) \\
            \quad \textbullet \quad \text{q's  intervals}($[q\_interval_1,q\_interval_2]$)
            
          \State {\bf Initialize:} 
            \If{$q\_interval_2[0] \neq \infty$}
                \State $q_{max} = max(q\_interval_1[1],q\_interval_2[1])$ \Comment{}
            \Else
                \State $q_{max} = q\_interval_1[1]$
            \EndIf
            \If{$q_{max} \neq 0$}
                \State \Return $[[p,N_c,K],[\epsilon,\delta],\gamma,q_{max}]$
            \Else
                \State \Return None
            \EndIf
        \EndProcedure
        \end{algorithmic}
    \end{algorithm} 
    \item \textbf{Compute accumulate noise}: After that, we compute the actual number of round $T$ using the equation $\frac{K}{N_c} = \sum_{i=0}^{T} q_i = sum_{i=0}^{T} q(i+m)^p$ and then compute the accumulate noise $\sigma \sqrt{T}$:
    \begin{algorithm}[H]
    \caption{Compute accumulate noise}
    \label{alg:ComputeAccumulateNoise}
        \begin{algorithmic}[1]
 \Procedure{$compute\_accumulate\_noise$}{$p,N_c,K,\epsilon,\delta,\sigma,\gamma,q\_max$}
            \State {\bf Input:} \\
            \quad \textbullet \quad $p \in [0,1]$, Dataset Size ($N_c$), Number of iterations (K) \\
            \quad \textbullet \quad $Privacy\ Budget(\epsilon,\delta), Gaussian\ Noise (\sigma)$ \\
            \quad \textbullet \quad $\gamma, q_{max}$
          \State {\bf Initialize:} 
            \State $i=0$
            \State $T_{max},m = compute\_sequence(p,N_c,K,q,\gamma)$
            \State $sum_q = 0$
            \While{$\frac{K}{N_c} > sum_q$}
                \State $sum_q = sum_q + q_{max} \cdot (i+m)^p$
                \State $i=i+1$
            \EndWhile
            \State $T = i - 1$ 
            \If{$T \leq \frac{1}{1+\gamma}((p+1)\frac{K}{s})^{1/(1+p)}$ or $T > T_{max}$}
                \State \Return None
            \EndIf
            \State \Return $[[p,N_c,K],[\epsilon,\delta],\sigma,[m,q_{max},T], \sigma \cdot \sqrt{T}]$
            \EndProcedure
        \end{algorithmic}
    \end{algorithm}
    The value of $T_{max}$ and $m$ is computed by the algorithm \ref{alg:ComputeSequence}:
    \begin{algorithm}
    \caption{Compute sequence}
    \label{alg:ComputeSequence}
        \begin{algorithmic}[1]
        \Procedure{$compute\_sequence$}{$p,N_c,K,q,\gamma$}
            \State {\bf Input:} \\
            \quad \textbullet \quad $p \in [0,1]$, Dataset Size ($N_c$), Number of iterations (K) \\
            \quad \textbullet \quad $q,\gamma$ 
          \State {\bf Initialize:} 
            \State $s = q \cdot N_c$
            \State $T_{max} = (\frac{(p+1) \cdot K}{q \cdot N_c})^\frac{1}{1+p}$
            \State $s_{0,c} = (\gamma \cdot T)^p \cdot s$
            \State $m = (\frac{s_{0,c}}{s})^{1/p}$
            \State \Return $T_{max}$,m
            \EndProcedure
        \end{algorithmic}
    \end{algorithm}
    \item \textbf{Select smallest accumulate noise}: Finally, we reduce the table size by choosing the smallest accumulate noise:
    \begin{algorithm}[H]
    \caption{Select smallest accumulate noise}
    \label{alg:SelectSmallestAccumulateNoise}
        \begin{algorithmic}[1]
        \Procedure{$select\_smallest\_accumulate\_noise$}{$p,N_c,K,Inverse\_table$}
            \State {\bf Input:} \\
            \quad \textbullet \quad $p \in [0,1]$, Dataset Size ($N_c$), Number of iterations (K) \\
            \quad \textbullet \quad $Inverse\_table(p,N_c,K)$
            \State {\bf Initialize:} 
            \State $SAN\_table =[]$
            \State $privacy\_budget\_groups = Inverse\_table.groupby([\epsilon,\delta])$ \Comment{Divide inverse table into privacy budget groups}
            \For{$group \in privacy\_budget\_groups$}
                \For{$row \in group$} 
                % \Comment{$row = [\sigma,[m,q_{max},T], accum\_noise]$}
                    \State $SAN = \infty$ \Comment{SAN = smallest accumulate noise}
                    \State $accum\_noise = row[2]$
                    \If{$SAN > accum\_noise$}
                        \State $SAN =  accum\_noise$
                        \State $row_{SAN} = row$
                    \EndIf
                \EndFor
                \State $SAN\_table.append(row_{SAN})$
            \EndFor
            \State \Return $SAN\_table$
        \EndProcedure
        \end{algorithmic}
    \end{algorithm}
\end{enumerate}

In our experiments, we generate the table entries for the number of epochs $K_{epochs} \in [1,100]$ and the Gaussian noise value $\sigma \in [1,\sigma_{max}]$ where $\sigma_{max}$ is choosing based on the sequential SGD with Gaussian noise and the accuracy degradation is $10\%$. Moreover, given $p,N_c,K,\epsilon,\delta,\sigma$, the value of $\gamma$ is bounded as follows:
\begin{itemize}
    \item Case 1: Since $\alpha = \frac{r_0}{\sigma} \geq 0$, we have the bound on $\gamma$:
    $\gamma \leq \left(\sigma \cdot \sqrt{\frac{\epsilon}{2\ln{1/\delta}}}\right)^{\frac{1}{2+3p}}-1$
    \item Case 2: According to \textbf{Theorem 6}, we have $\frac{K}{K^+} \geq 1$ and $r \geq \frac{\sqrt{3}-1}{2} \cdot \frac{(3p+1}{(p+1)(2p+1)} \cdot \frac{(1-\alpha)^2}{(1+\gamma)^{2p}}$. Then, we have the bound on $\gamma$ of case 2: 
    \[\gamma \leq \left(\frac{1}{1.21} \cdot \sigma \cdot \sqrt{\frac{\epsilon}{2\ln{1/\delta}}}\right)^{\frac{1}{2+3p}} -1 \leq \left(\sigma \cdot \sqrt{\frac{\epsilon}{2\ln{1/\delta}}}\right)^{\frac{1}{2+3p}}-1
    \]
\end{itemize}
Therefore, let $\gamma_{max} = \left(\sigma \cdot \sqrt{\frac{\epsilon}{2\ln{1/\delta}}}\right)^{\frac{1}{2+3p}}-1$, we use $\gamma \in [0,\gamma_{max}]$ in our calculator. After having all the components, we design the DP-calculator as follows:

\begin{algorithm}[H]
\caption{DP Calculator}
\label{alg:DPCalculator}
    \begin{algorithmic}[1]
    \Procedure{DP\_calculator}{$p,N_c,K,\epsilon_{array},\delta_{array},\sigma_{max}$}
        \State {\bf Input:} \\
        \quad \textbullet \quad p, Dataset size ($N_c$),number of iterations ($K$) \\
        \quad \textbullet \quad Privacy budgets ($\epsilon_{array},\delta_{array}$), Maximal Gaussian Noise ($\sigma_{max}$) 
        % \quad \textbullet \quad $\gamma$, \text{q's  intervals}($[qr_1,qr_2]$)
        % \quad \textbullet \quad SAN\_table
        \State {\bf Initialize:} 
        \State $inverse\_table = []$
        \For{$\epsilon \in \epsilon_{array}$}
            \For{$\delta \in \delta_{array}$}
                \For{$\sigma \in [1,\sigma_{max}]$}
                    \State $\gamma_{max} = \left(\sigma \cdot \sqrt{\frac{\epsilon}{2\ln{1/\delta}}}\right)^{\frac{1}{2+3p}}-1$
                    \For{$\gamma \in [0,\gamma_{max}]$}
                        \State $original\_table\_entry = construct\_original\_table(p,N_c,K,\epsilon,\delta,\sigma,\gamma)$
                        \If{ $\textbf{not}\ original\_table\_entry.isEmpty()$}
                            \State $q_{max} = compute\_q\_max(original\_table\_entry)[3]$
                            \State $inverse\_table\_entry = compute\_accumulate\_noise(p,N_c,K,\epsilon,\delta,\sigma,\gamma,q\_max)$
                            % \If{ $\textbf{not} inverse\_table\_entry.isEmpty()$}
                            \State $inverse\_table.append(inverse\_table\_entry)$
                            % \EndIf
                        \EndIf
                    \EndFor
                 \EndFor
            \EndFor
        \EndFor
        \State $SAN\_table = select\_smallest\_accumulate\_noise(p,N_c,K,inverse\_table)$
        \State \Return SAN\_table
        \EndProcedure
    \end{algorithmic}
\end{algorithm}

The next problem which we need to consider is choosing the value of K. If K is too large then we may not achieve the privacy because we leak too much information. Otherwise, the accuracy of the machine learning or deep learning model may be very low. Therefore, we use binary search on the "SAN\_table" to find the minimum $K = K_{min}$ such that an entry exists in this table given the privacy budget $(\epsilon,\delta)$.

Let $K_s$ be the standard number of iterations we need to achieve the accuracy we want on non-DP setting. We multiply $K_s$ by a factor of $\rho$ until we have an valid entry in the $SAN\_table$.
\begin{algorithm}[H]
\caption{Compute $K_{min}$}
    \begin{algorithmic}[1]
        \State {\bf Input:} \\
        \quad \textbullet \quad p, Dataset size ($N_c$), Standard number of iterations ($K_s$) \\
        \quad \textbullet \quad Privacy budgets ($\epsilon_{array},\delta_{array}$), Maximal Gaussian Noise ($\sigma_{max}$) \\
        \quad \textbullet \quad Multiplier Base ($\rho$)
        % \quad \textbullet \quad $\gamma$, \text{q's  intervals}($[qr_1,qr_2]$)
        % \quad \textbullet \quad SAN\_table
      \State {\bf Initialize:} 
        \State $i = 0$
        % \State $SAN\_table = DP\_calculator([p,N_c,K_{min}],[\epsilon_{array},\delta_{array},\sigma_{max}])$
        % \State $rows = SAN\_table.query(p,N_c,K_{min},\epsilon,\delta)$
        \Repeat
        \State $K_{min} = \rho^i \cdot K_s$
        \State $SAN\_table = DP\_calculator([p,N_c,K_{min}],[\epsilon_{array},\delta_{array},\sigma_{max}])$
        \State $rows = SAN\_table.query(p,N_c,K_{min},\epsilon,\delta)$
        \State $i=i+1$
        \Until{$rows$ is not empty}
        % \While{$row.isEmpty()$}
        %     \State $K_{min} = \rho^i \cdot K_s$
        %     \State $i=i+1$
        %     \State $SAN\_table = DP\_calculator([p,N_c,K_{min}],[\epsilon_{array},\delta_{array},\sigma_{max}])$
        %     \State $row = SAN\_table.query(p,N_c,K_{min},\epsilon,\delta)$
        % \EndWhile
        \State $row = rows[rows["\epsilon"] =rows["\epsilon"].min()]$ \Comment{Select row with smallest $\epsilon$}
        \State \Return [$K_{min},row$]
    \end{algorithmic}
\end{algorithm}

% \begin{algorithm}[H]
% \caption{Compute $K_{min}$}
%     \begin{algorithmic}[1]
%         \State {\bf Input:} \\
%         \quad \textbullet \quad p, Dataset size ($N_c$), Standard number of iterations ($K_s$) \\
%         \quad \textbullet \quad Privacy budget ($\epsilon,\delta$), Maximal Gaussian Noise ($\sigma_{max}$) 
%         % \quad \textbullet \quad $\gamma$, \text{q's  intervals}($[qr_1,qr_2]$)
%         % \quad \textbullet \quad SAN\_table
%       \State {\bf Initialize:} 
%         \State $K_{min} = K_s$
%         \State $i = 0, \rho = 2$
%         \State $row = []$
%         \While{$row.isEmpty()$}
%             \State $K_{min} = \rho^i \cdot K_s$
%             \State $SAN\_table = DP\_calculator([p,N_c,K_{min}],[\epsilon,\delta,\sigma_{max}])$
%             \If{ \textbf{not} SAN\_table\_entry.isEmpty()}
%                 \State $row = SAN\_table\_entry$
%             \EndIf
%             \State $i=i+1$
%         \EndWhile
%         \State \Return [$K_{min},row$]
%     \end{algorithmic}
% \end{algorithm}

However, $K=K_{min}$ may not be large enough to achieve the accuracy we want. Assuming there exists a value $K_{max}$ such that there is no valid entry in the "SAN\_table" for $K \geq K_{max}$, we can simply perform binary search on the interval $[K_{min},K_{max}]$ to find the optimal value $K = K_{opt}$ that has non-zero entry and acceptable accuracy. The algorithm \ref{alg:compute_K_max} shows how we compute the value of $K_{max}$.

% \begin{algorithm}[H]
% \caption{Compute $K_{max}$}
%     \begin{algorithmic}[1]
%         \State {\bf Input:} \\
%         \quad \textbullet \quad p, Dataset size ($N_c$), $K_{min}$ \\
%         \quad \textbullet \quad Privacy budget ($\epsilon,\delta$) \\
%         \quad \textbullet \quad SAN\_table
%       \State {\bf Initialize:} 
%         \State $K_{max} = K_{min}$
%         \State $i = 0, \rho = 2$
%         \State $row = SAN\_table.query(p,N_c,K_{max},\epsilon,\delta)$
%         \While{ \textbf{not} $row.isEmpty()$}
%             \State $K_{min} = \rho^i \cdot K_{min}$
%             \State $i=i+1$
%             \State $row = SAN\_table.query(p,N_c,K_{max},\epsilon,\delta)$
%         \EndWhile
%         \State \Return [$K_{max},row$]
%     \end{algorithmic}
%     \label{alg:compute_K_max}
% \end{algorithm}

\begin{algorithm}[H]
\caption{Compute $K_{max}$}
\label{alg:compute_K_max}
    \begin{algorithmic}[1]
        \State {\bf Input:} \\
        \quad \textbullet \quad p, Dataset size ($N_c$), Minimal number of iterations ($K_{min}$) \\
        \quad \textbullet \quad Privacy budgets ($\epsilon_{array},\delta_{array}$), Maximal Gaussian Noise ($\sigma_{max}$) \\
        \quad \textbullet \quad Multiplier Base ($\rho$)
        % \quad \textbullet \quad $\gamma$, \text{q's  intervals}($[qr_1,qr_2]$)
        % \quad \textbullet \quad SAN\_table
      \State {\bf Initialize:} 
        \State $i = 0$
        \Repeat
        \State $K_{max} = \rho^i \cdot K_{min}$
        \State $SAN\_table = DP\_calculator([p,N_c,K_{max}],[\epsilon_{array},\delta_{array},\sigma_{max}])$
        \State $rows = SAN\_table.query(p,N_c,K_{max},\epsilon,\delta)$
        \State $i=i+1$
        \Until{$rows$ is empty}
        \State \Return $K_{max}$
    \end{algorithmic}
\end{algorithm}
